# Supplementary material for: Acoustic Wavefront Manipulation: Impedance Inhomogeneity and Extraordinary Reflection
Source: arXiv:1301.0065 source file (2013-01-01)
Supplement: Supplementary file 1 [file Supplement.pdf]

# Supplement Material for "Acoustic Wavefront Manipulation: Impedance Inhomogeneity and Extraordinary Reflection"

Jiajun Zhao[1,2], Cheng-Wei Qiu[1], Zhining Chen[1], and Baowen Li[2,3]

[1]*Department of Electrical and Computer Engineering, National University of Singapore, Singapore 117576, Republic of Singapore*

[2]*Department of Physics and Centre for Computational Science and Engineering, National University of Singapore, Singapore 117546, Republic of Singapore and*

[3]*NUS-Tongji Center for Phononics and Thermal Energy Science, School of Physical Science and Engineering, Tongji University, Shanghai 200092, People's Republic of China*

(Dated: November 29, 2012)

## Abstract

This supplement material includes:

I. Derivation: The derivation of the proposed impedance governed Snell's law of reflection (IGSL) in acoustics

II. Simulation: One of the simulation in the case of the oblique acoustic plane-wave incidence

## I. DERIVATION

We assume the time-harmonic factor in this supplement is $e^{-i\omega t}$, where $\omega$ is the circular frequency, and the coordinate system is that in Fig. 1. The incident acoustic pressure can be expressed as:

$$p_i(y, z, \omega) = p_{i0}(\omega) \exp[ik_0(y \sin\theta_i - z \cos\theta_i)], \tag{1}$$

where $k_0 = \omega/c_0$ is the wave number in free space, $\theta_i$ the incident angle and $p_{i0}(\omega)$ the amplitude. We define $Z_n(y, \omega) \equiv p(y, 0, \omega)/[\mathbf{n} \cdot \mathbf{v}(y, 0, \omega)]$ ('$\equiv$': the symbol used for definition) as the specific acoustic impedance (SAI) [1] of a locally reacting boundary, where $\mathbf{n}$ is the unit vector opposite to $z$ direction and $\mathbf{v}$ is the acoustic velocity. The boundary condition of this problem can be paraphrased as [2]:

$$\frac{\partial}{\partial z} p(y, 0, \omega) + ik_0\beta(y, \omega)p(y, 0, \omega) = 0, \tag{2}$$

where $\beta(y, \omega) \equiv \rho_0 c_0/Z_n(y, \omega)$ ($\rho_0$ and $c_0$ being the given density and sound speed respectively in the upper space in Fig. 1) is the normalized acoustical admittance of the locally reacting surface.

We expand $\beta$ to be $\beta(y, \omega) = \tilde{\beta}(y, \omega) + \beta_0(\omega)$, where $\beta_0$ is a real constant. Thus the ordinary reflected wave contributed by $\beta_0$ is expressed as:

$$p_{r1}(y, z, \omega) = p_{i0}(\omega)R(\theta_i) \exp[ik_0(y \sin\theta_{r1} + z \cos\theta_{r1})], \tag{3}$$

where $R(\theta_i)$ is introduced as the reflection coefficient and $\theta_{r1}$ the angle of the ordinary reflection. Because the ordinary reflected wave observes the usual Snell's law, we know $\theta_{r1} = \vartheta_i$. In order to find the expression of $R(\theta_i)$, we introduce the constant SAI:

$$Z_0(\omega) = \frac{\rho_0 c_0}{\beta_0(\omega)} = \frac{p_i(y, 0, \omega) + p_{r1}(y, 0, \omega)}{\mathbf{n} \cdot \mathbf{v}_i(y, 0, \omega) + \mathbf{n} \cdot \mathbf{v}_{r1}(y, 0, \omega)}, \tag{4}$$

where $\mathbf{n}$ is the normal vector indicated in Fig. 1, $\mathbf{v}_i$ the acoustic velocity of the incident wave and $\mathbf{v}_{r1}$ the acoustic velocity of the ordinary reflection. Substituting Eq.(1) and Eq.(3) into Eq.(4) and applying the linearized Euler equation $\rho_0 \frac{\partial}{\partial t}\mathbf{v} = -\nabla p$, we reach the expression of $R$:

$$R(\theta_i) = \frac{\cos\theta_i - \beta_0(\omega)}{\cos\theta_i + \beta_0(\omega)}. \tag{5}$$

According to Eq.(3) and Eq.(5), it can be seen that the ordinary reflected wave contributed by the SAI $\beta_0$ will vanish if $\beta_0$ is set to be $\cos\theta_i$.

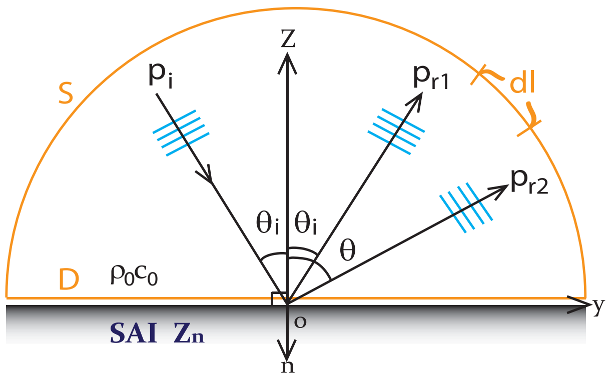


FIG. 1. Illustration for some notations. The orange line indicates the contour of the Green's integral. $S$ is the semicircular contour; $D$ is the flat one along the surface. $p_i$, $p_{r1}$ and $p_{r2}$ denote the incident wave, the ordinary reflected one contributed by the SAI $\beta_0$, and the extraordinary reflected one respectively. $\mathbf{n}$ is the unit vector opposite to $z$ direction. The SAI is $\rho_0 c_0$ for the upper space ($z > 0$), and $Z_n$ for the flat interface ($z = 0$).

In Fig. 1, there are no exciting sources in the upper space. Thanks to no sources inside the dash contour $S + D$, the total acoustic field can be written in the integral form:

$$p(y,z,\omega) = \oint_{S+D} [G(y,z,\omega;y_0,z_0)\frac{\partial}{\partial n_0}p(y_0,z_0,\omega) - p(y_0,z_0,\omega)\frac{\partial}{\partial n_0}G(y,z,\omega;y_0,z_0)]dl, \quad (6)$$

where $dl(y_0, z_0)$ is the infinitesimal length along the integral contour, $\mathbf{n}_0 \equiv \mathbf{n}(y_0, z_0)$ and $G(y, z, \omega; y_0, z_0)$ is the Green's function corresponding to the following partial differential problem:

$$\begin{array}{l} \nabla^2 G + {k_0}^2 G = -\delta(y-y_0)\delta(z-z_0), z > 0 \\ [\frac{\partial}{\partial z_0}G + ik_0\beta_0(\omega)G]\Big|_{z_0=0} = 0 \end{array}. \quad (7)$$

When the radius of the semicircular contour $S$ approaches $\infty$, we can regard the contour integral along $S$ is mainly contributed by $p_i$ and $p_{r1}$. Therefore Eq.(6) is altered into

$$p(y,z,\omega) = p_i(y,z,\omega) + p_{r1}(y,z,\omega) - \int_D [G\frac{\partial}{\partial z_0}p(y_0,z_0,\omega) - p(y_0,z_0,\omega)\frac{\partial}{\partial z_0}G]dy_0. \quad (8)$$

When the radius of the semicircular contour $S$ approaches $\infty$, the length of the flat contour $D$ will approach $\infty$ as well, in which case the upper and the lower limits of the definite integral in Eq.(8) can be changed into $\infty$ and $-\infty$ respectively. Therefore, we can simplify Eq.(8) by substituting Eq.(7) and Eq.(2) into it and simultaneously change the limits. Therefore

we obtain

$$p(y,z,\omega) = p_i(y,z,\omega) + p_{r1}(y,z,\omega) + ik_0 \int_{-\infty}^{\infty} \tilde{\beta}(y_0,\omega) p_0(y_0,0,\omega) G(y,z,\omega;y_0,0) dy_0. \quad (9)$$

Here we define the last part of Eq.(9) as the extra reflected wave $p_{r2}(y,z,\omega)$.

In addition, the explicit solution of $G(y,z,\omega;y_0,z_0)$ in terms of Eq.(7) is

$$G = \frac{i}{4} H_0^{(1)}(k_0 |\mathbf{r} - \mathbf{r}_0|) + \frac{i}{4\pi} \int_{-\infty}^{\infty} \frac{1}{k_z} \frac{k_z - \omega\beta_0/c_0}{k_z + \omega\beta_0/c_0} \exp[ik_z(z+z_0) + ik_y(y-y_0)] dk_y, \quad (10)$$

where $\mathbf{r} \equiv (y,z)$, $\mathbf{r}_0 \equiv (y,z)$, $k_0 \equiv \omega/c_0$ and ${k_0}^2 = {k_y}^2 + {k_z}^2$. When $\mathbf{r}$ is over one wavelength away from the surface $D$, it can be approximated that $k_z \approx k_0 \cos\theta^*$, where $\theta^*$ is introduced and the meaning of $\theta^*$ will be clarified later. Via this approximation and another definition $\mathbf{r}_0^\dagger \equiv (y_0, -z_0)$, it turns out that [3]

$$\cos\theta^* \approx \frac{z - (-z_0)}{\left|\mathbf{r} - \mathbf{r}_0^\dagger\right|} \approx constant. \quad (11)$$

The reason why $\cos\theta^*$ can be treated as a constant will be explained later, together with the meaning of $\theta^*$. By the approximation Eq.(11), it can be obtained that

$$\frac{k_z - \omega\beta_0/c_0}{k_z + \omega\beta_0/c_0} \approx \frac{\cos\theta^* - \beta_0(\omega)}{\cos\theta^* + \beta_0(\omega)} \approx constant \approx R(\theta^*). \quad (12)$$

Applying Eq.(12) into Eq.(10) and using the formula of the cylindrical wave expansion in terms of plane waves, we approach a neat form of the Green's function:

$$G(y,z,\omega;y_0,z_0) \approx \frac{i}{4} H_0^{(1)}(k_0 |\mathbf{r} - \mathbf{r}_0|) + R(\theta^*) \frac{i}{4} H_0^{(1)}(k_0 \left|\mathbf{r} - \mathbf{r}_0^\dagger\right|), \quad (13)$$

where $H_0^{(1)}(\cdot)$ the Hankel function of the first kind. We identify that $\frac{i}{4} H_0^{(1)}(k_0 |\mathbf{r} - \mathbf{r}_0|)$ is the two-dimensional Green's function excited by a point source in free space, which satisfies the analog of the three-dimensional case [4].

From the physical insight into Eq.(13), the first part of $G(y,z,\omega;y_0,z_0)$ can be interpreted as the direct contribution of the point source to the observer through path 2 in Fig. 2. The second part is the product of the Green's function excited by the image source and the reflection coefficient (the effect of the boundary), denoting the ordinary reflected wave. According to our interpretation, Fig. 2 illustrates path 1 and path 2, which are visualized as the incident wave and the ordinary reflected one respectively [5]. Due to the expression of the reflection coefficient, we figure out that $\theta^*$ is the effective incident angle regarding to

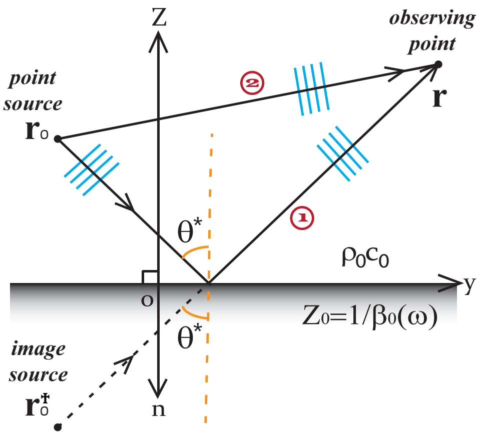


FIG. 2. Schematic diagram for the effective paths of acoustic radiation in the far field. The introduced $\theta^*$ can be interpreted as the effective incident angle. $\mathbf{r}$, $\mathbf{r}_0$, and $\mathbf{r}_0^\dagger$ are the location vectors for the point source, the image source and the observing point, respectively.

Fig. 2. Furthermore, it is reasonable to say that the major contribution of the integral in Eq.(10) is attributed to the vicinity of $\theta^*$, in which way $R(\theta^*)$ can be regarded as a constant and put outside the integral.

As for the far-field approximation, we are able to get the expansions as follows:

$$\begin{aligned} \mathbf{r}\cdot\mathbf{r}_0 &= r(y_0\sin\theta + z_0\cos\theta) \\ \mathbf{r}\cdot\mathbf{r}_0^\dagger &= r(y_0\sin\theta - z_0\cos\theta) \\ H_0^{(1)}(x)\Big|_{x\to\infty} &\approx \sqrt{\tfrac{2}{\pi x}}e^{i(x-\frac{\pi}{4})}, \end{aligned} \tag{14}$$

where $r$ is the length of $\mathbf{r}$, $\sin\theta = y/r$, and $\cos\theta = z/r$. Substituting Eq.(14) into Eq.(13), we obtain the far-field expression of $G(y,z,\omega;y_0,z_0)$:

$$G(y,z,\omega;y_0,z_0) \approx \frac{i}{4}\sqrt{\frac{2}{\pi k_0 r}}e^{i(k_0 r-\frac{\pi}{4})}e^{-ik_0 y_0\sin\theta}[e^{-ik_0 z_0\cos\theta} + R(\theta^*)e^{ik_0 z_0\cos\theta}]. \tag{15}$$

Because the Green's function is evaluated along the boundary, after setting $z_0 = 0$ and substituting Eq.(5) into Eq.(15), we get

$$G(y,z,\omega;y_0,0) \approx i\sqrt{\frac{1}{2\pi k_0 r}}e^{i(k_0 r-\frac{\pi}{4})}e^{-ik_0 y_0\sin\theta}\frac{\cos\theta^*}{\cos\theta^* + \beta_0(\omega)}. \tag{16}$$

Then after substituting Eq.(16) into $p_{r2}(y,z,\omega)$ in Eq.(9), the integral equation of $p_{r2}$ is derived as:

$$p_{r2}(y,z,\omega) \approx -\sqrt{\frac{k_0}{2\pi r}}e^{i(k_0 r-\frac{\pi}{4})}\frac{\cos\theta^*}{\cos\theta^* + \beta_0(\omega)}\int_{-\infty}^{\infty}\tilde{\beta}(y_0,\omega)p_0(y_0,0,\omega)e^{-ik_0 y_0\sin\theta}dy_0. \tag{17}$$

In order to solve $p_{r2}$ explicitly, we apply Born approximation $p(y_0, 0, \omega) \approx p_i(y_0, 0, \omega) + p_{r1}(y_0, 0, \omega)$ into Eq.(17) and expand it by Eq.(1) and Eq.(3). Then $p_{r2}(y, z, \omega)$ is transformed into a new form:

$$p_{r2} \approx -\sqrt{\frac{2k_0}{\pi r}} \frac{p_{i0}(\omega) \exp[i(k_0 r - \frac{\pi}{4})] \cos\theta^* \cos\theta_i}{[\cos\theta^* + \beta_0(\omega)][\cos\theta_i + \beta_0(\omega)]} \int_{-\infty}^{\infty} \tilde{\beta}(y_0, \omega) e^{ik_0 y_0 (\sin\theta_i - \sin\theta)} dy_0. \tag{18}$$

We can further define

$$\Psi^*(\theta, \omega) \equiv \int_{-\infty}^{\infty} \tilde{\beta}(y, \omega) e^{ik_0(\sin\theta_i - \sin\theta) y} dy, \tag{19}$$

which is with respect to the radiation angle. It is apparent to detect that Eq.(19) stands for the spatial Fourier transform $F\{\tilde{\beta}\}$.

Now we consider our proposed SAI in the main text:

$$Z_n(y, \omega) = A \frac{1}{\cos[\psi(y)/2]} e^{-i\psi(y)/2}. \tag{20}$$

After substituting it into $\beta(y, \omega)$, we get

$$\beta(y, \omega) - \beta_0(\omega) = \frac{\rho_0 c_0}{2A} e^{i\psi(y)} + \frac{\rho_0 c_0}{2A} - \beta_0(\omega). \tag{21}$$

Substituting Eq.(21) in Eq.(19), we approach

$$\Psi^*(\theta, \omega) = \int_{-\infty}^{\infty} \frac{\rho_0 c_0}{2A} e^{i\psi(y)} e^{i\frac{\omega}{c_0}(\sin\theta_i - \sin\theta) y} dy + \int_{-\infty}^{\infty} \left(\frac{\rho_0 c_0}{2A} - \beta_0\right) e^{i\frac{\omega}{c_0}(\sin\theta_i - \sin\theta) y} dy, \tag{22}$$

which yields

$$\Psi^*(\theta, \omega) = \frac{\rho_0 c_0}{2A} \delta[k_0 y(\sin\theta_i - \sin\theta) + \psi(y)] + \left(\frac{\rho_0 c_0}{2A} - \beta_0\right) \delta[k_0 y(\sin\theta_i - \sin\theta)]. \tag{23}$$

The first Dirac Delta function of Eq.(23) indicates the existence of the extraordinary reflection, while the second one indicates the contribution of the ordinary reflection. In order to shed light on the extraordinary reflection contributed by the first Dirac Delta, we define the first integral of Eq.(22) as $\Psi$, the directivity factor of the extraordinary reflection:

$$\Psi(\theta_{re}, \omega) \equiv \int_{-\infty}^{\infty} \frac{\rho_0 c_0}{2A} e^{i\psi(y)} e^{i\frac{\omega}{c_0}(\sin\theta_i - \sin\theta_{re}) y} dy = \frac{\rho_0 c_0}{2A} \delta[k_0 y(\sin\theta_i - \sin\theta_{re}) + \psi(y)], \tag{24}$$

where $\theta_{re}$ is the angle of the extraordinary reflection. The Dirac Delta function makes sense only when

$$k_0 y(\sin\theta_{re} - \sin\theta_i) = \psi(y). \tag{25}$$

Differentiating both sides of Eq.(25), we come to the final conclusion:

$$\sin\theta_{re} - \sin\theta_i = \frac{1}{k_0}\frac{d\psi(y)}{dy}, \tag{26}$$

which corresponds to the form of the generalized Snell's law of reflection (GSL) [6]. We name Eq.(26) as the impedance governed Snell's law of reflection (IGSL) in acoustics.

According to Eq.(3), we let $\beta_0(\omega) = \cos\theta_i$ so as to make $p_{r1}$, which is attributed by $\beta_0$, vanish. Besides, in order to suppress the partial ordinary reflection contributed by the second integral in Eq.(23), we set $A = \frac{\rho_0 c_0}{2\beta_0}$, i.e., $A = \frac{\rho_0 c_0}{2\cos\theta_i}$. Therefore Eq.(20) becomes

$$Z_n(y,\omega) = \frac{\rho_0 c_0}{2\cos\theta_i}\frac{1}{\cos[\psi(y)/2]}e^{-i\psi(y)/2}, \tag{27}$$

in which case the ordinary reflection disappears, only leaving the extraordinary reflection, and IGSL still holds.

## II. SIMULATION

In Fig. 3, we assume water ($\rho_0 = 1kg/m^3$; $c_0 = 1500m/s$ [1]) as the medium in the upper space. The SAI Eq.(27) with the linear parameter $\psi(y) = (10 + 10\sqrt{3})y$ is set along the flat surface, and an audible ($\omega = 30Krad/s$) plane wave with a unit amplitude is obliquely incident with the incident angle $-60°$. These parameters theoretically lead to the angle of extraordinary reflection $30°$ according to our proposed IGSL Eq.(26). Furthermore, the ordinary reflection vanishes thanks to the specific $A$ chosen in Eq.(27). In Fig. 3, we find the simulation by COMSOL® confirms the prediction via IGSL accurately, and ordinary reflection disappears as expected. Moreover, the incident audible plane wave and the extraordinary reflected wave are at the same side of the normal line, confirming the possibility of the negative extraordinary reflection. The singularity due to $\tan[\psi(y)/2]$ in the imaginary part of Eq. (20) does not play a significant role because the mathematical singularity $\pm i\infty$ just occurs to singular positions and means the total reflection (reflection coefficient equals $+1$).


[1] D. T. Blackstock, *Fundamentals of physical acoustics* (Wiley, 2000).

[2] M. A. Nobile, and S. I. Hayek, J. Acoust. Soc. Am. **78**, 1325 (1985).

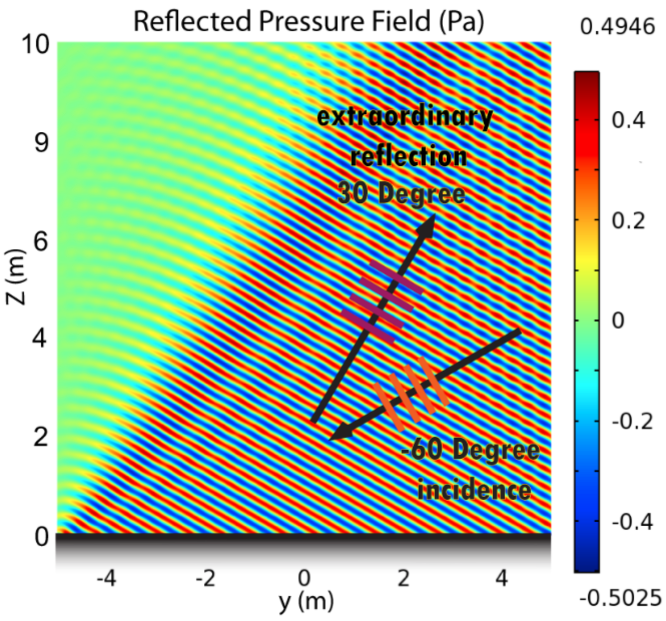


FIG. 3. The SAI Eq.(27) with $\psi(y) = (10 + 10\sqrt{3})y$ is set along the flat surface $z = 0$. In the upper space, the medium is water ($\rho_0 = 1kg/m^3$; $c_0 = 1500m/s$). An audible plane wave with unit amplitude and $\omega = 30Krad/s$ is $-60°$ obliquely incident. Only reflected acoustic pressure is plotted. The propagating path of the extraordinary reflection is noted as an arrow with purple crossbars.

[3] G. Taraldsen, J. Acoust. Soc. Am. **117**, 3389 (2005).

[4] C. F. Chien, and W. W. Soroka, J. Sound Vibrat. **43**, 9 (1975).

[5] G. Taraldsen, Wave Motion **43**, 91 (2005).

[6] N. Yu *et al.*, Science **334**, 333 (2011).
